# Supplementary material for: SAINT: Spatially Aware Interpolation NeTwork for Medical Slice Synthesis
Source: arXiv:2001.00704 source file (2020-01-03)
Supplement: Supplementary file 1 [file supplemental_img.tex]

\begin{figure*}[!htb]
    \setlength{\abovecaptionskip}{3pt}
    \setlength{\tabcolsep}{1pt}
    \centering
        \begin{tabular}[b]{c c c c c c c}
            \begin{subfigure}[b]{0.15\linewidth}
                \setlength{\abovecaptionskip}{1pt}
                \includegraphics[width=\linewidth,height=0.94\textwidth,cframe=red]{visualization_imgs/supplemental/liver_137/x4/ax/hr_big.png}
                \caption*{Ground Truth}
            \end{subfigure}
            &
            % \hspace{-2pt}
            \begin{subfigure}[b]{0.07\linewidth}
                \setlength{\abovecaptionskip}{3pt}
                \includegraphics[width=\linewidth,height=2\textwidth,cframe=red]{visualization_imgs/supplemental/liver_137/x4/ax/hr.png}
                \caption*{HR}
            \end{subfigure}
            &
            % \hspace{-2pt}
            \begin{subfigure}[b]{0.14\linewidth}
                \setlength{\abovecaptionskip}{2.5pt}
                \includegraphics[width=\linewidth,height=\textwidth,cframe=red]{visualization_imgs/supplemental/liver_137/x4/ax/bicu.png}
                \caption*{Bicubic}
            \end{subfigure}
            &
            % \hspace{-2pt}
            \begin{subfigure}[b]{0.14\linewidth}
                \setlength{\abovecaptionskip}{2.5pt}
                \includegraphics[width=\linewidth,height=\textwidth,cframe=red]{visualization_imgs/supplemental/liver_137/x4/ax/mdcsrn.png}
                \caption*{mDCSRN}
            \end{subfigure}
            &
            % \hspace{-2pt}
            \begin{subfigure}[b]{0.14\linewidth}
                \setlength{\abovecaptionskip}{2.5pt}
                \includegraphics[width=\linewidth,height=\textwidth,cframe=red]{visualization_imgs/supplemental/liver_137/x4/ax/mdsr.png}
                \caption*{3D MDSR}
            \end{subfigure}
            &
            % \hspace{-21pt}
            \begin{subfigure}[b]{0.14\linewidth}
                \setlength{\abovecaptionskip}{2.5pt}
                \includegraphics[width=\linewidth,height=\textwidth,cframe=red]{visualization_imgs/supplemental/liver_137/x4/ax/msr.png}
                \caption*{3D RDN}
            \end{subfigure}
            &
            % \hspace{-10pt}
            \begin{subfigure}[b]{0.15\linewidth}
                \setlength{\abovecaptionskip}{2.5pt}
                \includegraphics[width=\linewidth,height=0.94\textwidth,cframe=red]{visualization_imgs/supplemental/liver_137/x4/ax/saint.png}
                \caption*{SAINT}
            \end{subfigure}\\
            \begin{subfigure}[b]{0.15\linewidth}
                \setlength{\abovecaptionskip}{1pt}
                \includegraphics[width=\linewidth,height=0.94\textwidth,cframe=red]{visualization_imgs/supplemental/liver_137/x4/sag/hr_big.png}
                \caption*{Ground Truth}
            \end{subfigure}
            &
            % \hspace{-2pt}
            \begin{subfigure}[b]{0.07\linewidth}
                \setlength{\abovecaptionskip}{3pt}
                \includegraphics[width=\linewidth,height=2\textwidth,cframe=red]{visualization_imgs/supplemental/liver_137/x4/sag/hr.png}
                \caption*{HR}
            \end{subfigure}
            &
            % \hspace{-2pt}
            \begin{subfigure}[b]{0.14\linewidth}
                \setlength{\abovecaptionskip}{2.5pt}
                \includegraphics[width=\linewidth,height=\textwidth,cframe=red]{visualization_imgs/supplemental/liver_137/x4/sag/bicu.png}
                \caption*{Bicubic}
            \end{subfigure}
            &
            % \hspace{-2pt}
            \begin{subfigure}[b]{0.14\linewidth}
                \setlength{\abovecaptionskip}{2.5pt}
                \includegraphics[width=\linewidth,height=\textwidth,cframe=red]{visualization_imgs/supplemental/liver_137/x4/sag/mdcsrn.png}
                \caption*{mDCSRN}
            \end{subfigure}
            &
            % \hspace{-2pt}
            \begin{subfigure}[b]{0.14\linewidth}
                \setlength{\abovecaptionskip}{2.5pt}
                \includegraphics[width=\linewidth,height=\textwidth,cframe=red]{visualization_imgs/supplemental/liver_137/x4/sag/mdsr.png}
                \caption*{3D MDSR}
            \end{subfigure}
            &
            % \hspace{-21pt}
            \begin{subfigure}[b]{0.14\linewidth}
                \setlength{\abovecaptionskip}{2.5pt}
                \includegraphics[width=\linewidth,height=\textwidth,cframe=red]{visualization_imgs/supplemental/liver_137/x4/sag/msr.png}
                \caption*{3D RDN}
            \end{subfigure}
            &
            % \hspace{-10pt}
            \begin{subfigure}[b]{0.15\linewidth}
                \setlength{\abovecaptionskip}{2.5pt}
                \includegraphics[width=\linewidth,height=0.94\textwidth,cframe=red]{visualization_imgs/supplemental/liver_137/x4/sag/saint.png}
                \caption*{SAINT}
            \end{subfigure}\\            
            \begin{subfigure}[b]{0.15\linewidth}
                \setlength{\abovecaptionskip}{1pt}
                \includegraphics[width=\linewidth,height=0.94\textwidth,cframe=red]{visualization_imgs/supplemental/liver_176/x4/ax/hr_big.png}
                \caption*{Ground Truth}
            \end{subfigure}
            &
            % \hspace{-2pt}
            \begin{subfigure}[b]{0.07\linewidth}
                \setlength{\abovecaptionskip}{3pt}
                \includegraphics[width=\linewidth,height=2\textwidth,cframe=red]{visualization_imgs/supplemental/liver_176/x4/ax/hr.png}
                \caption*{HR}
            \end{subfigure}
            &
            % \hspace{-2pt}
            \begin{subfigure}[b]{0.14\linewidth}
                \setlength{\abovecaptionskip}{2.5pt}
                \includegraphics[width=\linewidth,height=\textwidth,cframe=red]{visualization_imgs/supplemental/liver_176/x4/ax/bicu.png}
                \caption*{Bicubic}
            \end{subfigure}
            &
            % \hspace{-2pt}
            \begin{subfigure}[b]{0.14\linewidth}
                \setlength{\abovecaptionskip}{2.5pt}
                \includegraphics[width=\linewidth,height=\textwidth,cframe=red]{visualization_imgs/supplemental/liver_176/x4/ax/mdcsrn.png}
                \caption*{mDCSRN}
            \end{subfigure}
            &
            % \hspace{-2pt}
            \begin{subfigure}[b]{0.14\linewidth}
                \setlength{\abovecaptionskip}{2.5pt}
                \includegraphics[width=\linewidth,height=\textwidth,cframe=red]{visualization_imgs/supplemental/liver_176/x4/ax/mdsr.png}
                \caption*{3D MDSR}
            \end{subfigure}
            &
            % \hspace{-21pt}
            \begin{subfigure}[b]{0.14\linewidth}
                \setlength{\abovecaptionskip}{2.5pt}
                \includegraphics[width=\linewidth,height=\textwidth,cframe=red]{visualization_imgs/supplemental/liver_176/x4/ax/msr.png}
                \caption*{3D RDN}
            \end{subfigure}
            &
            % \hspace{-10pt}
            \begin{subfigure}[b]{0.15\linewidth}
                \setlength{\abovecaptionskip}{2.5pt}
                \includegraphics[width=\linewidth,height=0.94\textwidth,cframe=red]{visualization_imgs/supplemental/liver_176/x4/ax/saint.png}
                \caption*{SAINT}
            \end{subfigure}\\
            \begin{subfigure}[b]{0.15\linewidth}
                \setlength{\abovecaptionskip}{1pt}
                \includegraphics[width=\linewidth,height=0.94\textwidth,cframe=red]{visualization_imgs/supplemental/liver_176/x4/sag/hr_big.png}
                \caption*{Ground Truth}
            \end{subfigure}
            &
            % \hspace{-2pt}
            \begin{subfigure}[b]{0.07\linewidth}
                \setlength{\abovecaptionskip}{3pt}
                \includegraphics[width=\linewidth,height=2\textwidth,cframe=red]{visualization_imgs/supplemental/liver_176/x4/sag/hr.png}
                \caption*{HR}
            \end{subfigure}
            &
            % \hspace{-2pt}
            \begin{subfigure}[b]{0.14\linewidth}
                \setlength{\abovecaptionskip}{2.5pt}
                \includegraphics[width=\linewidth,height=\textwidth,cframe=red]{visualization_imgs/supplemental/liver_176/x4/sag/bicu.png}
                \caption*{Bicubic}
            \end{subfigure}
            &
            % \hspace{-2pt}
            \begin{subfigure}[b]{0.14\linewidth}
                \setlength{\abovecaptionskip}{2.5pt}
                \includegraphics[width=\linewidth,height=\textwidth,cframe=red]{visualization_imgs/supplemental/liver_176/x4/sag/mdcsrn.png}
                \caption*{mDCSRN}
            \end{subfigure}
            &
            % \hspace{-2pt}
            \begin{subfigure}[b]{0.14\linewidth}
                \setlength{\abovecaptionskip}{2.5pt}
                \includegraphics[width=\linewidth,height=\textwidth,cframe=red]{visualization_imgs/supplemental/liver_176/x4/sag/mdsr.png}
                \caption*{3D MDSR}
            \end{subfigure}
            &
            % \hspace{-21pt}
            \begin{subfigure}[b]{0.14\linewidth}
                \setlength{\abovecaptionskip}{2.5pt}
                \includegraphics[width=\linewidth,height=\textwidth,cframe=red]{visualization_imgs/supplemental/liver_176/x4/sag/msr.png}
                \caption*{3D RDN}
            \end{subfigure}
            &
            % \hspace{-10pt}
            \begin{subfigure}[b]{0.15\linewidth}
                \setlength{\abovecaptionskip}{2.5pt}
                \includegraphics[width=\linewidth,height=0.94\textwidth,cframe=red]{visualization_imgs/supplemental/liver_176/x4/sag/saint.png}
                \caption*{SAINT}
            \end{subfigure}\\        
            \begin{subfigure}[b]{0.15\linewidth}
                \setlength{\abovecaptionskip}{1pt}
                \includegraphics[width=\linewidth,height=0.94\textwidth,cframe=red]{visualization_imgs/supplemental/liver_199/x4/ax/hr_big.png}
                \caption*{Ground Truth}
            \end{subfigure}
            &
            % \hspace{-2pt}
            \begin{subfigure}[b]{0.07\linewidth}
                \setlength{\abovecaptionskip}{3pt}
                \includegraphics[width=\linewidth,height=2\textwidth,cframe=red]{visualization_imgs/supplemental/liver_199/x4/ax/hr.png}
                \caption*{HR}
            \end{subfigure}
            &
            % \hspace{-2pt}
            \begin{subfigure}[b]{0.14\linewidth}
                \setlength{\abovecaptionskip}{2.5pt}
                \includegraphics[width=\linewidth,height=\textwidth,cframe=red]{visualization_imgs/supplemental/liver_199/x4/ax/bicu.png}
                \caption*{Bicubic}
            \end{subfigure}
            &
            % \hspace{-2pt}
            \begin{subfigure}[b]{0.14\linewidth}
                \setlength{\abovecaptionskip}{2.5pt}
                \includegraphics[width=\linewidth,height=\textwidth,cframe=red]{visualization_imgs/supplemental/liver_199/x4/ax/mdcsrn.png}
                \caption*{mDCSRN}
            \end{subfigure}
            &
            % \hspace{-2pt}
            \begin{subfigure}[b]{0.14\linewidth}
                \setlength{\abovecaptionskip}{2.5pt}
                \includegraphics[width=\linewidth,height=\textwidth,cframe=red]{visualization_imgs/supplemental/liver_199/x4/ax/mdsr.png}
                \caption*{3D MDSR}
            \end{subfigure}
            &
            % \hspace{-21pt}
            \begin{subfigure}[b]{0.14\linewidth}
                \setlength{\abovecaptionskip}{2.5pt}
                \includegraphics[width=\linewidth,height=\textwidth,cframe=red]{visualization_imgs/supplemental/liver_199/x4/ax/msr.png}
                \caption*{3D RDN}
            \end{subfigure}
            &
            % \hspace{-10pt}
            \begin{subfigure}[b]{0.15\linewidth}
                \setlength{\abovecaptionskip}{2.5pt}
                \includegraphics[width=\linewidth,height=0.94\textwidth,cframe=red]{visualization_imgs/supplemental/liver_199/x4/ax/saint.png}
                \caption*{SAINT}
            \end{subfigure}\\
            \begin{subfigure}[b]{0.15\linewidth}
                \setlength{\abovecaptionskip}{1pt}
                \includegraphics[width=\linewidth,height=0.94\textwidth,cframe=red]{visualization_imgs/supplemental/liver_199/x4/sag/hr_big.png}
                \caption*{Ground Truth}
            \end{subfigure}
            &
            % \hspace{-2pt}
            \begin{subfigure}[b]{0.07\linewidth}
                \setlength{\abovecaptionskip}{3pt}
                \includegraphics[width=\linewidth,height=2\textwidth,cframe=red]{visualization_imgs/supplemental/liver_199/x4/sag/hr.png}
                \caption*{HR}
            \end{subfigure}
            &
            % \hspace{-2pt}
            \begin{subfigure}[b]{0.14\linewidth}
                \setlength{\abovecaptionskip}{2.5pt}
                \includegraphics[width=\linewidth,height=\textwidth,cframe=red]{visualization_imgs/supplemental/liver_199/x4/sag/bicu.png}
                \caption*{Bicubic}
            \end{subfigure}
            &
            % \hspace{-2pt}
            \begin{subfigure}[b]{0.14\linewidth}
                \setlength{\abovecaptionskip}{2.5pt}
                \includegraphics[width=\linewidth,height=\textwidth,cframe=red]{visualization_imgs/supplemental/liver_199/x4/sag/mdcsrn.png}
                \caption*{mDCSRN}
            \end{subfigure}
            &
            % \hspace{-2pt}
            \begin{subfigure}[b]{0.14\linewidth}
                \setlength{\abovecaptionskip}{2.5pt}
                \includegraphics[width=\linewidth,height=\textwidth,cframe=red]{visualization_imgs/supplemental/liver_199/x4/sag/mdsr.png}
                \caption*{3D MDSR}
            \end{subfigure}
            &
            % \hspace{-21pt}
            \begin{subfigure}[b]{0.14\linewidth}
                \setlength{\abovecaptionskip}{2.5pt}
                \includegraphics[width=\linewidth,height=\textwidth,cframe=red]{visualization_imgs/supplemental/liver_199/x4/sag/msr.png}
                \caption*{3D RDN}
            \end{subfigure}
            &
            % \hspace{-10pt}
            \begin{subfigure}[b]{0.15\linewidth}
                \setlength{\abovecaptionskip}{2.5pt}
                \includegraphics[width=\linewidth,height=0.94\textwidth,cframe=red]{visualization_imgs/supplemental/liver_199/x4/sag/saint.png}
                \caption*{SAINT}
            \end{subfigure}\\                    
        \end{tabular}
    \caption{Visual comparisons of different methods against SAINT for $r_z = 4$. The difference maps are provided to the right of the results for better visualization. %For mDCSRN, distortion due to stitching smaller 3D patches are visible, as indicated by the red arrows. 
    Images are best viewed when magnified.} \label{fig:supp_visual_x4}
    %(a) is an slice from the Kidney dataset. Despite lower PSNR value compare to RDN, SAINT generates much clearer details. (b) is a slice from the Hepatic Vessels dataset. Note that the mDCSRN result has some minor artifact due to stitching individually infered 3D cubes together
    \vspace{-1em}
\end{figure*}
